# Supplementary material for: Effective Field Theory for Rydberg Polaritons
Source: arXiv:1605.05651 source file (2016-08-15)
Supplement: Supplementary file 1 [file RydEFT_Lett_supp.pdf]

# Supplemental Material to the Manuscript: "Effective Field Theory for Rydberg Polaritons"

## Contents


**I. Microscopic Model** 1

**II. Effective Range Corrections** 2
1. Weak Attractive Interactions 2
2. Strong Attractive Interactions 3

**III. EFT Including Raman Resonances** 3

**IV. Non-Perturbative $N$-body Interaction Potential** 3

**References** 5


## I. MICROSCOPIC MODEL

In this section, we derive the two-body Lippmann-Schwinger equation for an inhomogeneous density and show that the spatially varying scattering length $a(z)$ is well defined when the density varies slowly compared to the blockade radius.

The effective Hamiltonian, including decay, that describes the Rydberg polariton system is ($\hbar = 1$)

$$H = -ic \int dz\, \hat{\mathcal{E}}^\dagger(z)\partial_z \hat{\mathcal{E}}(z) - \int dz\, g_c(z)\big[\hat{\mathcal{P}}(z)\hat{\mathcal{E}}^\dagger(z) + h.c.\big] + H_p + H_{\rm int}, \tag{S1}$$

$$H_p = -\int dz (\Delta + i\gamma)\hat{\mathcal{P}}^\dagger(z)\hat{\mathcal{P}}(z) - i\gamma_s \hat{\mathcal{S}}^\dagger(z)\hat{\mathcal{S}}(z) - \Omega[\hat{\mathcal{P}}^\dagger(z)\hat{S}(z) + h.c.], \tag{S2}$$

$$H_{\rm int} = \int dz dz' V(z-z')\hat{S}^\dagger(z)\hat{S}^\dagger(z')\hat{S}(z')\hat{S}(z), \tag{S3}$$

where $\hat{\mathcal{E}}(z)$, $\hat{\mathcal{P}}(z)$, and $\hat{S}(z)$ are bosonic annihilation operators for a photon, excited atom, and Rydberg state at position $z$. They satisfy $[\hat{\mathcal{E}}(z), \hat{\mathcal{E}}^\dagger(z')] = [\hat{\mathcal{P}}(z), \hat{\mathcal{P}}^\dagger(z')] = [\hat{S}(z), \hat{S}^\dagger(z')] = \delta(z - z')$. The parameters $\Delta$, $\Omega$, $\gamma$, and $g_c(z)$ are defined in the main text and $\gamma_s$ is the halfwidth of the $s$-state.

For an inhomogeneous medium it is convenient to solve the scattering problem in real space. For a single polariton we can find the propagator at frequency $\omega$ from the equations of motion

$$-i\omega E(z) = -c\partial_z E + ig_c(z)P(z), \tag{S4}$$

$$-i\omega P(z) = -(\gamma - i\Delta)P(z) + ig_c(z)E(z) + i\Omega\, S(z), \tag{S5}$$

$$-i\omega S(z) = -\gamma_s S(z) + i\Omega P(z). \tag{S6}$$

The solution is given by

$$E_\omega(z, z_0) = \frac{1}{N_\omega(z)} \exp\left[i\int_{z_0}^{z} dz' q(\omega, z')\right], \tag{S7}$$

$$q(\omega, z) = \frac{\omega}{c}\left(1 - \frac{[g_c(z)]^2}{\tilde{\Delta}\tilde{\delta}}\right), \tag{S8}$$

$$P_\omega(z, z_0) = -\frac{g_c(z)}{\tilde{\Delta}}\left(1 + \frac{\Omega^2}{\tilde{\Delta}\tilde{\delta}}\right)E_\omega(z, z_0), \tag{S9}$$

$$S_\omega(z, z_0) = \frac{g_c(z)\Omega}{\tilde{\Delta}\tilde{\delta}}E_\omega(z, z_0), \tag{S10}$$

where $\tilde{\Delta} = \Delta + \omega + i\gamma$, $\tilde{\delta} = -\Omega^2/\tilde{\Delta} + \omega + i\gamma_s$, $N_\omega(z)$ is a normalization constant chosen to satisfy $|E_\omega(z)|^2 + |P_\omega(z)|^2 + |S_\omega(z)|^2 = 1$, and $q(\omega, z)$ is defined in Eq. (1) in the main text for $\gamma = \gamma_s = 0$.

To each of these wavefunctions, we associate the operator

$$\hat{\psi}^\dagger_\omega(z_0) = \int dz \sqrt{\rho(\omega, z_0)}\big[E_\omega(z, z_0)\hat{\mathcal{E}}^\dagger(z) + P_\omega(z, z_0)\hat{\mathcal{P}}^\dagger(z) + S_\omega(z, z_0)\hat{S}^\dagger(z)\big]. \tag{S11}$$

where $\rho(\omega, z_0) = dq(\omega, z_0)/d\omega$ is the local density of states. For an infinite, homogeneous medium this operator creates a dark-state polariton [S1]. For a sufficiently slowly varying density, this field becomes approximately bosonic with the commutation relation

$$[\hat{\psi}_\omega(z_0), \hat{\psi}^\dagger_{\omega'}(z_0)] = \int dz \rho(\omega, z_0) e^{i\int_{z_0}^{z} dz'[q(\omega,z') - q(\omega',z')]} \approx \rho(\omega, z_0)\delta[q(\omega, z_0) - q(\omega', z_0)] = \delta(\omega - \omega'). \tag{S12}$$

When $\omega$ is on the Raman resonance $\tilde{\Delta}\tilde{\delta} = 0$, these solutions need to be treated with care because $E_\omega \to 0$ and these states do not propagate. The Raman resonance condition

$$\tilde{\Delta}\tilde{\delta} = (\omega + i\gamma_s)(\Delta + \omega + i\gamma) - \Omega^2 = 0 \tag{S13}$$

has the solutions

$$\omega_\pm = -\frac{\Delta + i(\gamma + \gamma_s)}{2} \pm \sqrt{\frac{[\Delta + i(\gamma + \gamma_s)]^2}{4} + \Omega^2 + (\gamma - i\Delta)\gamma_s}. \tag{S14}$$

We work in the limit of large $\Delta$ and small $\gamma_s$, where these resonances can be treated as if they were on the real axis. For these two eigenstates, $\hat{\psi}^\dagger_\pm(z_0) = P_\pm \hat{\mathcal{P}}^\dagger(z_0) + S_\pm \hat{S}^\dagger(z_0)$ with

$$P_\pm = \frac{\omega_\pm}{\sqrt{\Omega^2 + \omega_\pm^2}}, \tag{S15}$$

$$S_\pm = \frac{\Omega}{\sqrt{\Omega^2 + \omega_\pm^2}}. \tag{S16}$$

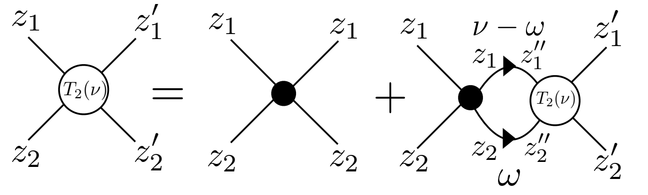

FIG. S1: Diagrammatic representation of the two-body Lippmann-Schwinger equation in real space, $\nu$ is the total frequency of the two polaritons, dots are $V(z_1 - z_2)$, and the lines are the single-polariton propagator $g_0^{ss}(z, z', \nu)$.

To solve the interacting problem, Eq. (S3) implies that we only need the propagator projected onto the Rydberg states. We can use the eigenstates $\psi_\omega^\dagger(z_0)|0\rangle$ to find the propagator in a vicinity of $z_0$

$$\begin{aligned} g_0^{ss}(z, z_0, \nu) &= \langle \hat{S}(z) \frac{1}{\nu - H_0 + i0^+} \hat{S}^\dagger(z_0) \rangle \quad \text{(S17)} \\ &= \int d\omega \frac{\langle \hat{S}(z)\psi_\omega^\dagger(z_0)\rangle \langle \psi_\omega(z_0)\hat{S}^\dagger(z_0)\rangle}{\nu - \omega + i0^+} \\ &= \rho(\nu, z_0) S_\nu(z, z_0) S_\nu^*(z_0, z_0) + \chi(\nu)\delta(z - z_0), \end{aligned}$$

$$\chi(\nu) = \sum_{s=\pm} \frac{|S_s|^2}{\nu - \omega_s} = \frac{\Delta + \nu}{(\Delta + \nu)\nu - \Omega^2}. \quad \text{(S18)}$$

As discussed in the main text, the $\chi(\nu)$ contribution arises from the two Raman resonances and accounts for the saturation of the propagator at large momentum.

With this representation of the single particle propagator, we can now write down the explicit Lippmann-Schwinger equation for the transition matrix for Rydberg polaritons in an inhomogeneous medium, represented diagrammatically in Fig. S1,

$$\begin{aligned} T_2(\boldsymbol{z}, \boldsymbol{z}', \nu) &= V(z_1 - z_2)\big[\delta(\boldsymbol{z} - \boldsymbol{z}') \quad \text{(S19)} \\ &+ \int d\boldsymbol{z}''\, g_0^{ss,ss}(\boldsymbol{z}, \boldsymbol{z}'', \nu) T_2(\boldsymbol{z}'', \boldsymbol{z}', \nu)\big], \\ g_0^{ss,ss}(\boldsymbol{z}, \boldsymbol{z}'', \nu) &= \int d\omega g_0^{ss}(z_1, z_1'', \omega) g_0^{ss}(z_2, z_2'', \nu - \omega). \quad \text{(S20)} \end{aligned}$$

To find the EFT parameters, we replace $g_0^{ss}(z_1, z_1'', \omega)$ with the first term in the last line of Eq. (S17) and approximate the dispersion by the formula given below Eq. (1) in the main text $\omega = v_g(z)q + q^2/2m(z)$. We then replace $V(z_1 - z_2)$ with the pseudopotential $-2\hbar^2\delta(r)/m(z)a(z)$, where $z = (z_1 + z_2)/2$ and $r = z_1 - z_2$ and derive an effective solution for $T_2$. This can then be matched to the asymptotic solution for the exact $T_2$. When the propagator varies slowly with $z$ compared to the potential (i.e., the density changes slowly on the scale of $r_b$), we can find $T_2$ using the anlysis of Ref. [S2] for a uniform density. In the next section, we discuss several regimes where $a$ can be found analytically with this approach.

## II. EFFECTIVE RANGE CORRECTIONS

In this section we give approximate formulas for the scattering length $a$ and effective range parameter $r_0$ at each scattering resonance for weak and strong attractive interactions.

These parameters can be found by solving the microscopic two-body problem using Eq. (S19). Assuming the density is slowly varying, we can make the local density approximation discussed in the main text and eliminate the center of mass momentum from Eq. (S19). In Ref. [S2], it was shown that the solution to the resulting integral equation can be found by solving a 1d Schrödinger-like equation

$$-\frac{1}{m}\partial_r^2\psi + V_{\text{eff}}^2(r)\psi = \nu\psi, \quad \text{(S21)}$$

where $r = z_1 - z_2$ is the relative distance between the two polaritons and $V_{\text{eff}}^2(r) = V(r)/[1 - \chi_2 V(r)]$ is shown in Fig. 3(e) in the main text. For $\chi_2 C_6 < 0$ the effective potential has no poles. In this case, the core of the potential, $r < r_b$, is approximately flat, while for $r > r_b$ it decays as $1/r^6$. The relative importance of the core versus the tail of the potential can be determined by comparing the associated length scales: the blockade radius $r_b$ versus the van der Waals length $r_{\text{vdw}} = (mC_6)^{1/4}$, respectively. Here we focus on the regime $\Omega \ll |\Delta|$, where $r_{\text{vdw}}$ can be expressed in terms of the interaction parameter $\varphi = g^2 r_b/c\Delta$ as $r_{\text{vdw}} \approx r_b\sqrt{\varphi}$. The scaling of $r_{\text{vdw}}$ with $\varphi$ indicates that, for weak interactions $\varphi \ll 1$, the low-energy scattering will be dominated by the core of the potential, while, for strong interactions $\varphi \gg 1$, the low-energy scattering will be dominated by the van der Waals tail. We now give approximate expressions for $a$ and $r_0$ in these two regimes for attractive interactions ($m/\chi_2 > 0$).

### 1. *Weak Attractive Interactions*

In the regime $\varphi \ll 1$, the low-energy scattering is dominated by the core of the potential, which can be well approximated by a square well of width $2r_b$. We parameterize the depth as $-\beta^2 r_b/\chi_2$, where $\beta$ is a free parameter chosen to match the observed scattering resonances. In this case, the scattering states can easily be found analytically and $a$ and $r_0$ take the form [S3]

$$a = r_b + \frac{r_b}{\beta\,\varphi\tan(\beta\,\varphi)}, \quad \text{(S22)}$$

$$\frac{r_0}{r_b} = 2 - 2\frac{r_b}{a} + \frac{2}{3}\frac{r_b^2}{a^2} - \left(1 - \frac{r_b}{a}\right)^2\left(\frac{\tan\beta\varphi}{\beta\varphi} + \frac{1}{\cos^2\beta\varphi}\right). \quad \text{(S23)}$$

In this approximation, the scattering resonances occur when $\varphi$ crosses $n\pi/\beta$. Expanding near each resonance

gives

$$n = 0,\ a = \frac{r_b}{\beta^2\varphi^2},\ \frac{r_0}{r_b} = \frac{2}{3}\,\beta^2\varphi^2, \tag{S24}$$

$$n > 0,\ a = \frac{r_b}{\beta n\pi\,\delta\varphi},\ \frac{r_0}{r_b} = 1 - \frac{\beta\delta\varphi}{n\pi}, \tag{S25}$$

where $\delta\varphi = \varphi - n\pi/\beta$ is assumed to be small.

We fix $\beta$ by comparing Eq. (S24) to the asymptotic result for $\varphi \to 0$. In this limit, one can replace the effective potential by a delta function $2v_0\,\delta(r)$, with $v_0 = \int_0^\infty dr V_{\rm eff}^2(r) = -(\pi/3)r_b/\chi_2$. The scattering length takes the form $a \approx (3/\pi)r_b/\varphi^2$ [S2], which fixes $\beta = \sqrt{\pi/3}$. With this choice of $\beta$, we find Eq. (S22) is in good agreement with the $n = 0$ and $n = 1$ scattering resonances characterized in Ref. [S2], but begins to deviate at the $n = 2$ scattering resonance.

### 2. *Strong Attractive Interactions*

When $\varphi \gg 1$, the effective potential for the polaritons has many features in common with the potentials considered in models of atomic scattering [S4]. In these models, the atomic potential $U(r)$ is treated as having a deep attractive core, while for large $r$

$$U(r) \approx -\frac{C_n}{r^n}, \tag{S26}$$

where $n = 6$ for van der Waals forces. For s-wave scattering, $a$ and $r_0$ can be found from the zero energy solution to the radial Schrödinger equation

$$\partial_r^2\psi_0 + [p(r)]^2\psi_0 = 0, \tag{S27}$$

where $p(r) = \sqrt{-mU(r)}$ and the boundary condition for s-wave scattering is $\psi_0(0) = 0$.

For the 1d Rydberg polariton problem considered here, Eq. (S27) is equivalent to Eq. (S21) with $p(r) = \varphi/\sqrt{r_b^2 + r^6/r_b^4}$, but with the boundary condition $\partial_r\psi_0|_{r=0} = 0$. Due to the similarity in the equations, for $\varphi \gg 1$, we can follow Ref. [S4, S5] to find analytical solutions for $a$ and $r_0$. In particular, we can solve for $\psi_0$ for small $r$ using a WKB approximation, which can then be matched to the known asymptotic solution for $\psi_0$ at large $r$. The WKB solution is valid in the region $r \ll \sqrt{\varphi}\,r_b$, while the asymptotic solution is valid when $r \gg r_b$ [S4]. Thus, the existence of an intermediate regime $r_b \ll r \ll \sqrt{\varphi}\,r_b$ is equivalent to the requirement of strong interactions $\varphi \gg 1$.

With these points in mind, we write the zero energy solution as

$$\psi_0(x) = \begin{cases} \dfrac{C}{\sqrt{p(r)}}\cos\left[\int_0^r dr' p(r')\right],\ r \ll \sqrt{\varphi}\,r_b \\ \sqrt{x}\left[AJ_{1/4}\left(\frac{\varphi\,r_b^2}{2\,r^2}\right) - BN_{1/4}\left(\frac{\varphi\,r_b^2}{2\,r^2}\right)\right],\ r \gg r_b \end{cases} \tag{S28}$$

where $A$, $B$, and $C$ are unkown coefficients which have to be determined by matching the two solutions in the intermediate region and $J_\alpha$ ($N_\alpha$) are Bessel functions of the first (second) kind. The WKB solution is chosen to satisfy the boundary condition that $\psi_0$ has zero derivative at the origin. Following a similar analysis to Ref. [S4, S5] we solve for the coefficients $A$, $B$, and $C$, which determine $a$ and $r_0$ as

$$a = \bar{a}\Big[1 - \tan\big(\Phi + \pi/8\big)\Big], \tag{S29}$$

$$\bar{a} = \frac{\Gamma(3/4)}{\Gamma(1/4)}\sqrt{2\,\varphi}\,r_b \approx 0.478\sqrt{\varphi}\,r_b, \tag{S30}$$

$$\Phi = \int_0^\infty drp(r) = \frac{\Gamma(1/3)\Gamma(7/6)}{\sqrt{\pi}}\varphi \approx 1.40\,\varphi, \tag{S31}$$

$$r_0 = 1.39\sqrt{\varphi}\,r_b - 1.333\frac{\varphi\,r_b^2}{a} + 0.637\frac{\varphi^{3/2}\,r_b^3}{a^2} \tag{S32}$$

where $\bar{a}$ is the scattering length averaged over $\Phi$ (excluding the resonances) and $\Gamma(\cdot)$ is the gamma function. The scattering resonances occur when $\Phi = \Phi_n = n\pi + 3\pi/8$. Expanding near the $n$th resonance gives

$$a \approx \frac{\bar{a}}{\Phi - \Phi_n}, \tag{S33}$$

while the effective range becomes $r_0 \approx 1.39\,r_{\rm vdw}$.

## III. EFT INCLUDING RAMAN RESONANCES

In this section, we write down an EFT that describes the coupling between the polariton field $\hat{\psi}$ and the Raman resonance excitations.

We account for the presence of the constant term in the propagator $g_0^{ss}(q,\nu)$ by adding a fictitious pair of particles $d_\pm$ to the EFT

$$\mathcal{H} = -\frac{1}{2m}\hat{\psi}^\dagger\partial_z^2\hat{\psi} + \sum_{s=\pm}\omega_s d_s^\dagger d_s \tag{S34}$$
$$+ \int dz'\Psi^\dagger(z)\Psi^\dagger(z')V(z-z')\Psi(z')\Psi(z),$$

$$\Psi(z) = \alpha\,\hat{\psi}(z) + S_+d_+(z) + S_-d_-(z), \tag{S35}$$

where $\omega_\pm$ is given by Eq. (S14) and the interaction term accounts for all of the allowed interactions between the fictitious particles. The terms $\alpha = g_c/\sqrt{\Omega^2 + g_c^2} \approx 1$ and $S_\pm$ (given by Eq. (S16)) account for the overlap of these particles with the $|s\rangle$ state. Integrating out the fields $d_\pm$ gives rise to the $N$-body interactions discussed in the main text and in the section below.

## IV. NON-PERTURBATIVE $N$-BODY INTERACTION POTENTIAL

When $|\chi_N V(r)| > 1$, the perturbative solution for $V_{\rm eff}^N$ given in Eq. (8) of the main text breaks down. We now

show how to find the non-perturbative solution to $V_{\rm eff}^N$ recursively using the Rosenberg integral equations for the connected transition matrix [S6]. We explicitly solve these equations for $N = 2$, 3, and 4. Finally, we show that, inside the blockade radius, $V_{\rm eff}^N$ oscillates between attraction and repulsion with every increase in $N$.

Before writing the Rosenberg equations, we first introduce some basic concepts needed to describe $N$-particle scattering [S7]. The notion of connected scattering diagrams, illustrated in Fig. 3 in the main text, leads to the cluster decomposition for the $N$-body transition matrix

$$T_N = \sum_{\alpha\in P}[T_N]_\alpha, \tag{S36}$$

where $P$ is the set of all partitions of $N$ particles into disjoint clusters. For example, for three particles there are five such partitions (1)(2)(3), (12)(3), (13)(2), (23)(1), and (123). We define $n_\alpha$ as the number of clusters within the partition $\alpha$. We denote the particles represented in each cluster as $i_1, \ldots, i_{m_n}$, where $1 \le n \le n_\alpha$ and $m_n$ is the length of the $n$th cluster. For the partition (12)(3) $n_\alpha = 2$, $m_1 = 2$ with $i_1 = 1, i_2 = 2$ and $m_2$=1 with $i_1 = 3$. We also introduce the notion of an ordering $\prec$ of the clusters: $\alpha \prec \beta$ if every cluster in $\alpha$ is a subset of the elements in clusters of $\beta$. For example, $(12)(3)(45) \prec (123)(456)$, but $(12)(3)(45) \not\prec (1234)(56)$.

To find each term in Eq. (S36), one needs to evaluate the sum of all scattering diagrams where each cluster in the partition is disconnected from the others, but fully connected internally. For example, the diagram in Fig. 3(b) of the main text contributes to $[T_N]_\alpha$ with $\alpha = (12)(345)$. In Eq. (8) of the main text we derived a perturbative solution for the fully connected contribution to $T_N$, $V_{\rm eff}^N = [T_N]_\alpha$ with $\alpha = (1, \ldots, N)$. However, this equation breaks down for $r \ll r_b$ where $|\chi_N V(r)| > 1$. In this limit, $V_{\rm eff}^N$ has to be found non-perturbatively.

The key insight into the connected $N$-body scattering diagrams is that they can each be written as the product $M_\alpha^\ell \chi_N L_\ell$, where $L_\ell$ is a diagram that ends with interaction $V_\ell$ on the left and $M_\alpha^\ell$ can be broken into two disjoint clusters $\alpha$ such that $\ell \not\prec \alpha$ [S8, S6]. For the connected diagram in Fig. 3(a) in the main text $M_\alpha^\ell = (\chi_N)^2 V_{12}V_{23}V_{24}$ and $L_\ell = V_{45}$, with $\alpha = (1234)(5)$ and $\ell = (45)$. The Rosenberg integral equations (which are algebraic equations for a constant propagator) take advantage of this structure to recursively define [S6, S7]

$$T_{N\ell}^c = \sum_{\ell'}\sum_{\alpha\succ\ell, n_\alpha=2}[T_\ell]_\alpha \bar{\Delta}_{\alpha\ell'}\chi_N T_{\ell'}, \tag{S37}$$

$$T_\ell = V_\ell + V_\ell\chi_N T_N = \frac{V_\ell}{1-\chi_N\sum_{\ell'}V_{\ell'}}, \tag{S38}$$

$$V_{\rm eff}^N(\boldsymbol{z};\nu) = \sum_\ell T_{N\ell}^c(\boldsymbol{z};\nu), \tag{S39}$$

where $T_N = \sum_\ell T_\ell$, $\ell = (ij)$ denotes a particle pair and ranges over all $N(N-1)/2$ pairs (note, we changed notation from Eq. (8) in the main text), $T_\ell$ groups all diagrams contributing to $T_N$ that end with the interaction $V_\ell$ on the left, and $\nu$ is the total frequency of the incoming photons. The sum in Eq. (S37) is over all partitions $\alpha$ with two clusters, which contain the pair $\ell$. The matrix $\bar{\Delta}_{\alpha\ell'} = 1$ if $\ell' \not\prec \alpha$ and zero otherwise. $\bar{\Delta}_{\alpha\ell'}$ reflects the structure of the connected diagrams described above and enforces that all the terms in Eq. (S37) are fully connected. Using the results from Sec. I, we can also give an explicit expression for the $N$-body propagator

$$\chi_N(\nu) = \sum_{\{(s_1,\ldots,s_N),s_i=\pm\}}\frac{1}{\nu-\sum_{i=1}^N\omega_{s_i}}\prod_{i=1}^N|S_{s_i}|^2. \tag{S40}$$

Equation (S37) is recursive because $[T_\ell]_\alpha$ can be expressed in terms of the connected transition matrices for $1 \le k \le N-2$

$$[T_\ell]_\alpha = T_{N-1,\ell}^{Nc}(z_{i_1},\ldots,z_{i_{N-1}}),\ (k=1) \tag{S41}$$

$$[T_\ell]_\alpha = \binom{N-3}{k-1}\chi_N T_{N-k,\ell}^{Nc}(z_{i_1},\ldots,z_{i_{N-k}}) \times \sum_{\ell'\prec(i_1\ldots i_k)}T_{k\ell'}^{Nc}(z_{i_1},\ldots,z_{i_k}), (k>1) \tag{S42}$$

where the superscript $N$ denotes that $T_{m\ell}^{Nc}$ is found using Eq. (S37) for $m$ particles, but with the propagator $\chi_N$ replacing $\chi_m$. The binomial factor in front of Eq. (S42) counts the number of ways to arrange the scattering events between the two clusters, with the constraint that the pair $\ell$ always interact first.

For $N = 3$, we find the non-perturbative solution

$$T_{3(12)}^c = \frac{\chi_3}{1-\chi_3\sum_\ell V_\ell}\frac{V_{12}}{1-\chi_3V_{12}}(V_{13}+V_{23}), \tag{S43}$$

$$T_{3(13)}^c = \frac{\chi_3}{1-\chi_3\sum_\ell V_\ell}\frac{V_{13}}{1-\chi_3V_{13}}(V_{12}+V_{23}), \tag{S44}$$

$$T_{3(23)}^c = \frac{\chi_3}{1-\chi_3\sum_\ell V_\ell}\frac{V_{23}}{1-\chi_3V_{23}}(V_{12}+V_{13}), \tag{S45}$$

$$V_{\rm eff}^3(z_1,z_2,z_3;\nu) = \sum_\ell T_{3\ell}^c(z_1,z_2,z_3;\nu), \tag{S46}$$

which agrees with the perturbative result from Eq. (8) in the main text to lowest order in $|\chi_3 V_\ell|$. For $N = 4$, the full expression involves considerably more terms:

$$\begin{aligned}T_{4(12)}^c = \frac{\chi_4}{1-\chi_4\sum_\ell V_\ell}\Big[&T_{3(12)}^{4c}(z_1,z_2,z_3)(V_{14}+V_{24}+V_{34})\\ &+T_{3(12)}^{4c}(z_1,z_2,z_4)(V_{13}+V_{23}+V_{34})\\ &+\chi_4T_{2(12)}^{4c}T_{2(34)}^{4c}(V_{13}+V_{14}+V_{23}+V_{24})\Big],\end{aligned} \tag{S47}$$

and similarly for the other $\ell$. Here $T_{3(12)}^{4c}(z_1,z_2,z_3)$ is given by $T_{3(12)}^c(z_1,z_2,z_3)$ from Eq. (S43) with $\chi_3(\nu)$ replaced by $\chi_4(\nu)$, $T_{2(12)}^{4c} = V_{12}/(1-\chi_4V_{12})$ and similarly for $T_{3(12)}^{4c}(z_1,z_2,z_4)$ and $T_{2(34)}^{4c}$. The resulting expression for $V_{\rm eff}^4$, to lowest order in $\chi_4 V_\ell$, contains 96 tree diagrams (16 unique) and agrees with Eq. (8) in the main text.

By construction, Eq. (S37) accounts for all connected scattering diagrams. To check that these recursive formulas give the same number of terms as the perturbative result, we use Eq. (S37)-(S42) to find a recursive formula for the number of terms contributing to $T^{c}_{N\ell}$

$$t_2^\ell = 1, \tag{S48}$$

$$t_N^\ell = t_{N-1}^\ell (N-2)(N-1) + \sum_{k=2}^{N-2} t_{N-k}^\ell t_k^\ell \frac{k(k-1)}{2} \binom{N-3}{k-1} \binom{N-2}{k} (N-k)k, \tag{S49}$$

where $\binom{N-2}{k}$ is the number two-cluster partitions containing $\ell$ with $m_1 = N-k$ and $m_2 = k$ and $(N-k)k$ is the number of non-zero elements in $\bar{\Delta}_{\alpha\ell'}$ for each two-cluster partition $\alpha$. Based on Eq. (8) in the main text we expect $t_N^\ell = 2(N-2)!N^{N-3}$. This can be proved by induction using Eq. (S49) combined with an application of the binomial formula [S9]

$$\frac{(a+b)^n}{a} = \sum_{k=0}^{n} \binom{n}{k} (a-kc)^{k-1} (b+kc)^{n-k}, \tag{S50}$$

with $a=1$, $c=-1$, $b=N-1$, and $n=N-3$. This result helps confirm that Eq. (8) of the main text is consistent with our non-perturbative solution for $V^N_{\text{eff}}$.

When all the photons are separated by much less than the blockade radius, we can approximate $V(r)$ by $\pm\infty$. In this limit, $T^{Nc}_{k\ell}$ saturates to a constant value that depends only on $N$ and $k$. By adapting the counting arguments used to derive Eq. (S49), after some simplifications, we then arrive at a similar recursive formula for $V^N_{\text{eff}}(z_1, \ldots, z_N; \nu)$ in this regime

$$V^N_{\text{eff}}(z_1, \ldots, z_N; \nu) \approx (-1)^{N-1} \frac{c_N}{\chi_N}, \tag{S51}$$

$$c_N = 2c_{N-1} + 2\sum_{k=2}^{N-2} \binom{N-3}{k-1} \binom{N-2}{k-1} c_{N-k} c_k, \tag{S52}$$

where $c_2 = 1$ and $c_3 = 2$. Since $c_N$ is a positive integer for every $N$, we find that, similar to the perturbative result from Eq. (10) in the main text, $V^N_{\text{eff}}$ alternates between attraction and repulsion for every increase in $N$.


[S1] M. Fleischhauer, A. Imamoglu, and J. P. Marangos, Rev. Mod. Phys. **77**, 633 (2005).
[S2] P. Bienias, S. Choi, O. Firstenberg, M. F. Maghrebi, M. Gullans, M. D. Lukin, A. V. Gorshkov, and H. P. Büchler, Phys. Rev. A **90**, 053804 (2014).
[S3] V. E. Barlette, M. M. Leite, and S. K. Adhikari, Eur. J. Phys. **21**, 435 (2000).
[S4] G. F. Gribakin and V. V. Flambaum, Phys. Rev. A **48**, 546 (1993).
[S5] V. V. Flambaum, G. F. Gribakin, and C. Harabati, Phys. Rev. A **59**, 1998 (1999).
[S6] L. Rosenberg, Phys. Rev. **140**, B217 (1965).
[S7] S. K. Adhikari and K. L. Kowalski, *Dynamical Collision Theory and Its Applications* (Academic Press, San Diego, CA, 1991).
[S8] S. Weinberg, Phys. Rev. **133**, B232 (1964).
[S9] R. P. Stanley, *Enumerative Combinatorics, Volume 1* (Cambridge Univ. Press, Cambridge, 2011), 2nd ed.
